# Supplementary material for: Color-Kinematic Duality in ABJM Theory Without Amplitude Relations
Source: arXiv:1402.1821 ancillary file (2014-02-08)
Supplement: Supplementary file 1 [file Amp_decomp_and_num_relations.pdf]

## 6 Attached PDF File: Explicit expressions at eight points

### A Amplitudes in terms of numerators

In the body of this note, we showed how to decompose the eight-point ABJM amplitudes into numerators. The amplitudes satisfy various symmetry properties, including KK-type relations. There are 57 amplitudes independent under these symmetries, and are expressed initially in terms of 216 numerators. We present a set of 57 basis amplitudes below.

$$\begin{aligned}
A(12345876) &= -\frac{n_1}{s_{123}s_{876}} - \frac{n_2}{s_{123}s_{587}} - \frac{n_7}{s_{123}s_{458}} + \frac{n_{28}}{s_{587}s_{612}} - \frac{n_{30}}{s_{458}s_{612}} - \frac{n_{36}}{s_{345}s_{612}} \\
&\quad - \frac{n_{136}}{s_{458}s_{761}} - \frac{n_{139}}{s_{345}s_{761}} + \frac{n_{144}}{s_{234}s_{761}} + \frac{n_{163}}{s_{234}s_{876}} + \frac{n_{164}}{s_{234}s_{587}} + \frac{n_{208}}{s_{345}s_{876}}, \\
A(12365478) &= \frac{n_5}{s_{123}s_{478}} - \frac{n_8}{s_{123}s_{547}} + \frac{n_9}{s_{123}s_{654}} + \frac{n_{48}}{s_{547}s_{812}} - \frac{n_{49}}{s_{654}s_{812}} - \frac{n_{51}}{s_{365}s_{812}} \\
&\quad + \frac{n_{154}}{s_{654}s_{781}} - \frac{n_{155}}{s_{365}s_{781}} + \frac{n_{160}}{s_{236}s_{781}} - \frac{n_{171}}{s_{236}s_{478}} + \frac{n_{173}}{s_{236}s_{547}} - \frac{n_{212}}{s_{365}s_{478}}, \\
A(12365874) &= \frac{n_2}{s_{123}s_{587}} - \frac{n_3}{s_{123}s_{658}} - \frac{n_5}{s_{123}s_{874}} + \frac{n_{11}}{s_{412}s_{587}} - \frac{n_{12}}{s_{412}s_{658}} - \frac{n_{18}}{s_{365}s_{412}} \\
&\quad - \frac{n_{100}}{s_{658}s_{741}} - \frac{n_{103}}{s_{365}s_{741}} + \frac{n_{107}}{s_{236}s_{741}} + \frac{n_{170}}{s_{236}s_{587}} + \frac{n_{171}}{s_{236}s_{874}} + \frac{n_{212}}{s_{365}s_{874}}, \\
A(12385476) &= \frac{n_6}{s_{123}s_{476}} + \frac{n_7}{s_{123}s_{854}} + \frac{n_8}{s_{123}s_{547}} + \frac{n_{30}}{s_{612}s_{854}} + \frac{n_{31}}{s_{547}s_{612}} - \frac{n_{33}}{s_{385}s_{612}} \\
&\quad + \frac{n_{136}}{s_{761}s_{854}} + \frac{n_{137}}{s_{385}s_{761}} + \frac{n_{142}}{s_{238}s_{761}} + \frac{n_{178}}{s_{238}s_{476}} + \frac{n_{179}}{s_{238}s_{547}} - \frac{n_{213}}{s_{385}s_{476}}, \\
A(12385674) &= \frac{n_3}{s_{123}s_{856}} + \frac{n_4}{s_{123}s_{567}} - \frac{n_6}{s_{123}s_{674}} + \frac{n_{12}}{s_{412}s_{856}} + \frac{n_{13}}{s_{412}s_{567}} - \frac{n_{17}}{s_{385}s_{412}} \\
&\quad + \frac{n_{100}}{s_{741}s_{856}} + \frac{n_{102}}{s_{385}s_{741}} + \frac{n_{106}}{s_{238}s_{741}} + \frac{n_{177}}{s_{238}s_{567}} - \frac{n_{178}}{s_{238}s_{674}} + \frac{n_{213}}{s_{385}s_{674}}, \\
A(14325678) &= \frac{n_{55}}{s_{143}s_{678}} - \frac{n_{58}}{s_{143}s_{567}} - \frac{n_{63}}{s_{143}s_{256}} + \frac{n_{109}}{s_{567}s_{814}} + \frac{n_{114}}{s_{256}s_{814}} - \frac{n_{117}}{s_{325}s_{814}} \\
&\quad - \frac{n_{158}}{s_{256}s_{781}} - \frac{n_{161}}{s_{325}s_{781}} - \frac{n_{162}}{s_{432}s_{781}} + \frac{n_{163}}{s_{432}s_{678}} - \frac{n_{166}}{s_{432}s_{567}} - \frac{n_{167}}{s_{325}s_{678}}, \\
A(14325876) &= -\frac{n_{55}}{s_{143}s_{876}} - \frac{n_{56}}{s_{143}s_{587}} - \frac{n_{61}}{s_{143}s_{258}} + \frac{n_{91}}{s_{587}s_{614}} - \frac{n_{95}}{s_{258}s_{614}} - \frac{n_{99}}{s_{325}s_{614}} \\
&\quad - \frac{n_{140}}{s_{258}s_{761}} - \frac{n_{143}}{s_{325}s_{761}} - \frac{n_{144}}{s_{432}s_{761}} - \frac{n_{163}}{s_{432}s_{876}} - \frac{n_{164}}{s_{432}s_{587}} + \frac{n_{167}}{s_{325}s_{876}},
\end{aligned}$$

$$\begin{aligned}
A(14365278) &= \frac{n_{59}}{s_{143}s_{278}} - \frac{n_{62}}{s_{143}s_{527}} + \frac{n_{63}}{s_{143}s_{652}} - \frac{n_{111}}{s_{365}s_{814}} + \frac{n_{113}}{s_{527}s_{814}} - \frac{n_{114}}{s_{652}s_{814}} \\
&\quad + \frac{n_{155}}{s_{365}s_{781}} + \frac{n_{156}}{s_{436}s_{781}} + \frac{n_{158}}{s_{652}s_{781}} + \frac{n_{195}}{s_{436}s_{527}} - \frac{n_{205}}{s_{278}s_{365}} - \frac{n_{206}}{s_{278}s_{436}}, \\
A(14365872) &= -\frac{n_{11}}{s_{214}s_{587}} + \frac{n_{12}}{s_{214}s_{658}} + \frac{n_{18}}{s_{214}s_{365}} - \frac{n_{37}}{s_{658}s_{721}} - \frac{n_{42}}{s_{365}s_{721}} + \frac{n_{44}}{s_{436}s_{721}} \\
&\quad + \frac{n_{56}}{s_{143}s_{587}} - \frac{n_{57}}{s_{143}s_{658}} - \frac{n_{59}}{s_{143}s_{872}} + \frac{n_{205}}{s_{365}s_{872}} + \frac{n_{206}}{s_{436}s_{872}} + \frac{n_{209}}{s_{436}s_{587}}, \\
A(14385276) &= \frac{n_{60}}{s_{143}s_{276}} + \frac{n_{61}}{s_{143}s_{852}} + \frac{n_{62}}{s_{143}s_{527}} - \frac{n_{93}}{s_{385}s_{614}} + \frac{n_{95}}{s_{614}s_{852}} + \frac{n_{96}}{s_{527}s_{614}} \\
&\quad - \frac{n_{137}}{s_{385}s_{761}} + \frac{n_{138}}{s_{438}s_{761}} + \frac{n_{140}}{s_{761}s_{852}} + \frac{n_{194}}{s_{438}s_{527}} - \frac{n_{201}}{s_{276}s_{385}} + \frac{n_{202}}{s_{276}s_{438}}, \\
A(14385672) &= -\frac{n_{12}}{s_{214}s_{856}} - \frac{n_{13}}{s_{214}s_{567}} + \frac{n_{17}}{s_{214}s_{385}} + \frac{n_{37}}{s_{721}s_{856}} + \frac{n_{41}}{s_{385}s_{721}} + \frac{n_{43}}{s_{438}s_{721}} \\
&\quad + \frac{n_{57}}{s_{143}s_{856}} + \frac{n_{58}}{s_{143}s_{567}} - \frac{n_{60}}{s_{143}s_{672}} + \frac{n_{201}}{s_{385}s_{672}} - \frac{n_{202}}{s_{438}s_{672}} + \frac{n_{211}}{s_{438}s_{567}}, \\
A(16325478) &= \frac{n_{65}}{s_{163}s_{478}} - \frac{n_{67}}{s_{163}s_{547}} - \frac{n_{72}}{s_{163}s_{254}} + \frac{n_{145}}{s_{547}s_{816}} + \frac{n_{150}}{s_{254}s_{816}} - \frac{n_{152}}{s_{325}s_{816}} \\
&\quad - \frac{n_{159}}{s_{254}s_{781}} - \frac{n_{160}}{s_{632}s_{781}} + \frac{n_{161}}{s_{325}s_{781}} - \frac{n_{168}}{s_{325}s_{478}} + \frac{n_{171}}{s_{478}s_{632}} - \frac{n_{173}}{s_{547}s_{632}}, \\
A(16325874) &= -\frac{n_{64}}{s_{163}s_{587}} - \frac{n_{65}}{s_{163}s_{874}} - \frac{n_{69}}{s_{163}s_{258}} - \frac{n_{91}}{s_{416}s_{587}} + \frac{n_{95}}{s_{258}s_{416}} + \frac{n_{99}}{s_{325}s_{416}} \\
&\quad - \frac{n_{104}}{s_{258}s_{741}} - \frac{n_{107}}{s_{632}s_{741}} - \frac{n_{108}}{s_{325}s_{741}} + \frac{n_{168}}{s_{325}s_{874}} - \frac{n_{170}}{s_{587}s_{632}} - \frac{n_{171}}{s_{632}s_{874}}, \\
A(16345278) &= \frac{n_{68}}{s_{163}s_{278}} - \frac{n_{70}}{s_{163}s_{527}} + \frac{n_{72}}{s_{163}s_{452}} - \frac{n_{147}}{s_{345}s_{816}} + \frac{n_{148}}{s_{527}s_{816}} - \frac{n_{150}}{s_{452}s_{816}} \\
&\quad - \frac{n_{156}}{s_{634}s_{781}} + \frac{n_{157}}{s_{345}s_{781}} + \frac{n_{159}}{s_{452}s_{781}} - \frac{n_{195}}{s_{527}s_{634}} + \frac{n_{206}}{s_{278}s_{634}} - \frac{n_{207}}{s_{278}s_{345}}, \\
A(16345872) &= -\frac{n_{28}}{s_{216}s_{587}} + \frac{n_{30}}{s_{216}s_{458}} + \frac{n_{36}}{s_{216}s_{345}} - \frac{n_{38}}{s_{458}s_{721}} - \frac{n_{44}}{s_{634}s_{721}} - \frac{n_{45}}{s_{345}s_{721}} \\
&\quad + \frac{n_{64}}{s_{163}s_{587}} - \frac{n_{66}}{s_{163}s_{458}} - \frac{n_{68}}{s_{163}s_{872}} - \frac{n_{206}}{s_{634}s_{872}} + \frac{n_{207}}{s_{345}s_{872}} - \frac{n_{209}}{s_{587}s_{634}}, \\
A(16385274) &= \frac{n_{69}}{s_{163}s_{852}} + \frac{n_{70}}{s_{163}s_{527}} + \frac{n_{71}}{s_{163}s_{274}} + \frac{n_{93}}{s_{385}s_{416}} - \frac{n_{95}}{s_{416}s_{852}} - \frac{n_{96}}{s_{416}s_{527}} \\
&\quad + \frac{n_{101}}{s_{638}s_{741}} - \frac{n_{102}}{s_{385}s_{741}} + \frac{n_{104}}{s_{741}s_{852}} + \frac{n_{186}}{s_{274}s_{638}} - \frac{n_{187}}{s_{274}s_{385}} + \frac{n_{193}}{s_{527}s_{638}}, \\
A(16385472) &= -\frac{n_{30}}{s_{216}s_{854}} - \frac{n_{31}}{s_{216}s_{547}} + \frac{n_{33}}{s_{216}s_{385}} + \frac{n_{38}}{s_{721}s_{854}} + \frac{n_{40}}{s_{638}s_{721}} - \frac{n_{41}}{s_{385}s_{721}} \\
&\quad + \frac{n_{66}}{s_{163}s_{854}} + \frac{n_{67}}{s_{163}s_{547}} - \frac{n_{71}}{s_{163}s_{472}} - \frac{n_{186}}{s_{472}s_{638}} + \frac{n_{187}}{s_{385}s_{472}} + \frac{n_{215}}{s_{547}s_{638}},
\end{aligned}$$

$$\begin{aligned}
A(18325476) &= \frac{n_{74}}{s_{183}s_{476}} + \frac{n_{75}}{s_{183}s_{547}} - \frac{n_{81}}{s_{183}s_{254}} - \frac{n_{141}}{s_{254}s_{761}} - \frac{n_{142}}{s_{761}s_{832}} + \frac{n_{143}}{s_{325}s_{761}} \\
&\quad - \frac{n_{145}}{s_{547}s_{618}} - \frac{n_{150}}{s_{254}s_{618}} + \frac{n_{152}}{s_{325}s_{618}} - \frac{n_{169}}{s_{325}s_{476}} - \frac{n_{178}}{s_{476}s_{832}} - \frac{n_{179}}{s_{547}s_{832}}, \\
A(18325674) &= \frac{n_{73}}{s_{183}s_{567}} - \frac{n_{74}}{s_{183}s_{674}} - \frac{n_{79}}{s_{183}s_{256}} - \frac{n_{105}}{s_{256}s_{741}} - \frac{n_{106}}{s_{741}s_{832}} + \frac{n_{108}}{s_{325}s_{741}} \\
&\quad - \frac{n_{109}}{s_{418}s_{567}} - \frac{n_{114}}{s_{256}s_{418}} + \frac{n_{117}}{s_{325}s_{418}} + \frac{n_{169}}{s_{325}s_{674}} - \frac{n_{177}}{s_{567}s_{832}} + \frac{n_{178}}{s_{674}s_{832}}, \\
A(18345276) &= \frac{n_{77}}{s_{183}s_{276}} + \frac{n_{78}}{s_{183}s_{527}} + \frac{n_{81}}{s_{183}s_{452}} - \frac{n_{138}}{s_{761}s_{834}} + \frac{n_{139}}{s_{345}s_{761}} + \frac{n_{141}}{s_{452}s_{761}} \\
&\quad + \frac{n_{147}}{s_{345}s_{618}} - \frac{n_{148}}{s_{527}s_{618}} + \frac{n_{150}}{s_{452}s_{618}} - \frac{n_{194}}{s_{527}s_{834}} - \frac{n_{202}}{s_{276}s_{834}} - \frac{n_{203}}{s_{276}s_{345}}, \\
A(18345672) &= -\frac{n_{39}}{s_{456}s_{721}} - \frac{n_{43}}{s_{721}s_{834}} + \frac{n_{45}}{s_{345}s_{721}} - \frac{n_{46}}{s_{218}s_{567}} - \frac{n_{49}}{s_{218}s_{456}} + \frac{n_{54}}{s_{218}s_{345}} \\
&\quad - \frac{n_{73}}{s_{183}s_{567}} - \frac{n_{76}}{s_{183}s_{456}} - \frac{n_{77}}{s_{183}s_{672}} + \frac{n_{202}}{s_{672}s_{834}} + \frac{n_{203}}{s_{345}s_{672}} - \frac{n_{211}}{s_{567}s_{834}}, \\
A(18365274) &= -\frac{n_{78}}{s_{183}s_{527}} + \frac{n_{79}}{s_{183}s_{652}} + \frac{n_{80}}{s_{183}s_{274}} - \frac{n_{101}}{s_{741}s_{836}} + \frac{n_{103}}{s_{365}s_{741}} + \frac{n_{105}}{s_{652}s_{741}} \\
&\quad + \frac{n_{111}}{s_{365}s_{418}} - \frac{n_{113}}{s_{418}s_{527}} + \frac{n_{114}}{s_{418}s_{652}} - \frac{n_{186}}{s_{274}s_{836}} - \frac{n_{188}}{s_{274}s_{365}} - \frac{n_{193}}{s_{527}s_{836}}, \\
A(18365472) &= \frac{n_{39}}{s_{654}s_{721}} - \frac{n_{40}}{s_{721}s_{836}} + \frac{n_{42}}{s_{365}s_{721}} - \frac{n_{48}}{s_{218}s_{547}} + \frac{n_{49}}{s_{218}s_{654}} + \frac{n_{51}}{s_{218}s_{365}} \\
&\quad - \frac{n_{75}}{s_{183}s_{547}} + \frac{n_{76}}{s_{183}s_{654}} - \frac{n_{80}}{s_{183}s_{472}} + \frac{n_{186}}{s_{472}s_{836}} + \frac{n_{188}}{s_{365}s_{472}} - \frac{n_{215}}{s_{547}s_{836}}, \\
A(12347856) &= \frac{n_2}{s_{123}s_{785}} - \frac{n_3}{s_{123}s_{856}} - \frac{n_5}{s_{123}s_{478}} - \frac{n_{28}}{s_{612}s_{785}} - \frac{n_{29}}{s_{478}s_{612}} - \frac{n_{35}}{s_{347}s_{612}} \\
&\quad - \frac{n_{118}}{s_{478}s_{561}} + \frac{n_{121}}{s_{347}s_{561}} + \frac{n_{126}}{s_{234}s_{561}} - \frac{n_{164}}{s_{234}s_{785}} + \frac{n_{165}}{s_{234}s_{856}} + \frac{n_{210}}{s_{347}s_{856}}, \\
A(12367458) &= \frac{n_6}{s_{123}s_{674}} + \frac{n_7}{s_{123}s_{458}} + \frac{n_8}{s_{123}s_{745}} - \frac{n_{47}}{s_{674}s_{812}} - \frac{n_{48}}{s_{745}s_{812}} - \frac{n_{50}}{s_{367}s_{812}} \\
&\quad + \frac{n_{127}}{s_{581}s_{674}} - \frac{n_{128}}{s_{367}s_{581}} + \frac{n_{134}}{s_{236}s_{581}} - \frac{n_{172}}{s_{236}s_{458}} - \frac{n_{173}}{s_{236}s_{745}} - \frac{n_{214}}{s_{367}s_{458}}, \\
A(12367854) &= -\frac{n_1}{s_{123}s_{678}} - \frac{n_2}{s_{123}s_{785}} - \frac{n_7}{s_{123}s_{854}} - \frac{n_{10}}{s_{412}s_{678}} - \frac{n_{11}}{s_{412}s_{785}} - \frac{n_{16}}{s_{367}s_{412}} \\
&\quad - \frac{n_{82}}{s_{541}s_{678}} + \frac{n_{85}}{s_{367}s_{541}} + \frac{n_{90}}{s_{236}s_{541}} - \frac{n_{170}}{s_{236}s_{785}} + \frac{n_{172}}{s_{236}s_{854}} + \frac{n_{214}}{s_{367}s_{854}}, \\
A(12387456) &= \frac{n_5}{s_{123}s_{874}} - \frac{n_8}{s_{123}s_{745}} + \frac{n_9}{s_{123}s_{456}} + \frac{n_{29}}{s_{612}s_{874}} - \frac{n_{31}}{s_{612}s_{745}} - \frac{n_{32}}{s_{387}s_{612}} \\
&\quad + \frac{n_{118}}{s_{561}s_{874}} + \frac{n_{119}}{s_{387}s_{561}} + \frac{n_{124}}{s_{238}s_{561}} - \frac{n_{179}}{s_{238}s_{745}} + \frac{n_{180}}{s_{238}s_{456}} - \frac{n_{216}}{s_{387}s_{456}},
\end{aligned}$$

$$\begin{aligned}
A(12387654) &= \frac{n_1}{s_{123}s_{876}} - \frac{n_4}{s_{123}s_{765}} - \frac{n_9}{s_{123}s_{654}} + \frac{n_{10}}{s_{412}s_{876}} - \frac{n_{13}}{s_{412}s_{765}} - \frac{n_{14}}{s_{387}s_{412}} \\
&\quad + \frac{n_{82}}{s_{541}s_{876}} + \frac{n_{83}}{s_{387}s_{541}} + \frac{n_{88}}{s_{238}s_{541}} - \frac{n_{177}}{s_{238}s_{765}} - \frac{n_{180}}{s_{238}s_{654}} + \frac{n_{216}}{s_{387}s_{654}}, \\
A(14327658) &= \frac{n_{57}}{s_{143}s_{658}} + \frac{n_{58}}{s_{143}s_{765}} - \frac{n_{60}}{s_{143}s_{276}} - \frac{n_{109}}{s_{765}s_{814}} + \frac{n_{112}}{s_{276}s_{814}} - \frac{n_{115}}{s_{327}s_{814}} \\
&\quad - \frac{n_{131}}{s_{276}s_{581}} - \frac{n_{133}}{s_{327}s_{581}} - \frac{n_{135}}{s_{432}s_{581}} + \frac{n_{165}}{s_{432}s_{658}} + \frac{n_{166}}{s_{432}s_{765}} - \frac{n_{174}}{s_{327}s_{658}}, \\
A(14327856) &= \frac{n_{56}}{s_{143}s_{785}} - \frac{n_{57}}{s_{143}s_{856}} - \frac{n_{59}}{s_{143}s_{278}} - \frac{n_{91}}{s_{614}s_{785}} - \frac{n_{94}}{s_{278}s_{614}} - \frac{n_{98}}{s_{327}s_{614}} \\
&\quad - \frac{n_{122}}{s_{278}s_{561}} + \frac{n_{125}}{s_{327}s_{561}} - \frac{n_{126}}{s_{432}s_{561}} + \frac{n_{164}}{s_{432}s_{785}} - \frac{n_{165}}{s_{432}s_{856}} + \frac{n_{174}}{s_{327}s_{856}}, \\
A(14367258) &= \frac{n_{60}}{s_{143}s_{672}} + \frac{n_{61}}{s_{143}s_{258}} + \frac{n_{62}}{s_{143}s_{725}} - \frac{n_{110}}{s_{367}s_{814}} - \frac{n_{112}}{s_{672}s_{814}} - \frac{n_{113}}{s_{725}s_{814}} \\
&\quad + \frac{n_{128}}{s_{367}s_{581}} + \frac{n_{130}}{s_{436}s_{581}} + \frac{n_{131}}{s_{581}s_{672}} - \frac{n_{195}}{s_{436}s_{725}} - \frac{n_{197}}{s_{258}s_{367}} - \frac{n_{199}}{s_{258}s_{436}}, \\
A(14367852) &= \frac{n_{10}}{s_{214}s_{678}} + \frac{n_{11}}{s_{214}s_{785}} + \frac{n_{16}}{s_{214}s_{367}} - \frac{n_{19}}{s_{521}s_{678}} + \frac{n_{24}}{s_{367}s_{521}} + \frac{n_{27}}{s_{436}s_{521}} \\
&\quad - \frac{n_{55}}{s_{143}s_{678}} - \frac{n_{56}}{s_{143}s_{785}} - \frac{n_{61}}{s_{143}s_{852}} + \frac{n_{197}}{s_{367}s_{852}} + \frac{n_{199}}{s_{436}s_{852}} - \frac{n_{209}}{s_{436}s_{785}}, \\
A(14387256) &= \frac{n_{59}}{s_{143}s_{872}} - \frac{n_{62}}{s_{143}s_{725}} + \frac{n_{63}}{s_{143}s_{256}} - \frac{n_{92}}{s_{387}s_{614}} + \frac{n_{94}}{s_{614}s_{872}} - \frac{n_{96}}{s_{614}s_{725}} \\
&\quad - \frac{n_{119}}{s_{387}s_{561}} + \frac{n_{120}}{s_{438}s_{561}} + \frac{n_{122}}{s_{561}s_{872}} - \frac{n_{190}}{s_{256}s_{387}} + \frac{n_{191}}{s_{256}s_{438}} - \frac{n_{194}}{s_{438}s_{725}}, \\
A(14387652) &= -\frac{n_{10}}{s_{214}s_{876}} + \frac{n_{13}}{s_{214}s_{765}} + \frac{n_{14}}{s_{214}s_{387}} + \frac{n_{19}}{s_{521}s_{876}} + \frac{n_{22}}{s_{387}s_{521}} + \frac{n_{25}}{s_{438}s_{521}} \\
&\quad + \frac{n_{55}}{s_{143}s_{876}} - \frac{n_{58}}{s_{143}s_{765}} - \frac{n_{63}}{s_{143}s_{652}} + \frac{n_{190}}{s_{387}s_{652}} - \frac{n_{191}}{s_{438}s_{652}} - \frac{n_{211}}{s_{438}s_{765}}, \\
A(16327458) &= \frac{n_{66}}{s_{163}s_{458}} + \frac{n_{67}}{s_{163}s_{745}} - \frac{n_{71}}{s_{163}s_{274}} - \frac{n_{132}}{s_{274}s_{581}} + \frac{n_{133}}{s_{327}s_{581}} - \frac{n_{134}}{s_{581}s_{632}} \\
&\quad - \frac{n_{145}}{s_{745}s_{816}} + \frac{n_{149}}{s_{274}s_{816}} - \frac{n_{151}}{s_{327}s_{816}} + \frac{n_{172}}{s_{458}s_{632}} + \frac{n_{173}}{s_{632}s_{745}} - \frac{n_{175}}{s_{327}s_{458}}, \\
A(16327854) &= \frac{n_{64}}{s_{163}s_{785}} - \frac{n_{66}}{s_{163}s_{854}} - \frac{n_{68}}{s_{163}s_{278}} - \frac{n_{86}}{s_{278}s_{541}} + \frac{n_{89}}{s_{327}s_{541}} - \frac{n_{90}}{s_{541}s_{632}} \\
&\quad + \frac{n_{91}}{s_{416}s_{785}} + \frac{n_{94}}{s_{278}s_{416}} + \frac{n_{98}}{s_{327}s_{416}} + \frac{n_{170}}{s_{632}s_{785}} - \frac{n_{172}}{s_{632}s_{854}} + \frac{n_{175}}{s_{327}s_{854}}, \\
A(16347258) &= \frac{n_{69}}{s_{163}s_{258}} + \frac{n_{70}}{s_{163}s_{725}} + \frac{n_{71}}{s_{163}s_{472}} + \frac{n_{129}}{s_{347}s_{581}} - \frac{n_{130}}{s_{581}s_{634}} + \frac{n_{132}}{s_{472}s_{581}} \\
&\quad - \frac{n_{146}}{s_{347}s_{816}} - \frac{n_{148}}{s_{725}s_{816}} - \frac{n_{149}}{s_{472}s_{816}} + \frac{n_{195}}{s_{634}s_{725}} - \frac{n_{198}}{s_{258}s_{347}} + \frac{n_{199}}{s_{258}s_{634}},
\end{aligned}$$

$$\begin{aligned}
A(16347852) &= -\frac{n_{20}}{s_{478}s_{521}} + \frac{n_{26}}{s_{347}s_{521}} - \frac{n_{27}}{s_{521}s_{634}} + \frac{n_{28}}{s_{216}s_{785}} + \frac{n_{29}}{s_{216}s_{478}} + \frac{n_{35}}{s_{216}s_{347}} \\
&\quad - \frac{n_{64}}{s_{163}s_{785}} - \frac{n_{65}}{s_{163}s_{478}} - \frac{n_{69}}{s_{163}s_{852}} + \frac{n_{198}}{s_{347}s_{852}} - \frac{n_{199}}{s_{634}s_{852}} + \frac{n_{209}}{s_{634}s_{785}}, \\
A(16387254) &= \frac{n_{68}}{s_{163}s_{872}} - \frac{n_{70}}{s_{163}s_{725}} + \frac{n_{72}}{s_{163}s_{254}} - \frac{n_{83}}{s_{387}s_{541}} + \frac{n_{84}}{s_{541}s_{638}} + \frac{n_{86}}{s_{541}s_{872}} \\
&\quad + \frac{n_{92}}{s_{387}s_{416}} - \frac{n_{94}}{s_{416}s_{872}} + \frac{n_{96}}{s_{416}s_{725}} - \frac{n_{182}}{s_{254}s_{387}} + \frac{n_{183}}{s_{254}s_{638}} - \frac{n_{193}}{s_{638}s_{725}}, \\
A(16387452) &= \frac{n_{20}}{s_{521}s_{874}} - \frac{n_{22}}{s_{387}s_{521}} + \frac{n_{23}}{s_{521}s_{638}} - \frac{n_{29}}{s_{216}s_{874}} + \frac{n_{31}}{s_{216}s_{745}} + \frac{n_{32}}{s_{216}s_{387}} \\
&\quad + \frac{n_{65}}{s_{163}s_{874}} - \frac{n_{67}}{s_{163}s_{745}} - \frac{n_{72}}{s_{163}s_{452}} + \frac{n_{182}}{s_{387}s_{452}} - \frac{n_{183}}{s_{452}s_{638}} - \frac{n_{215}}{s_{638}s_{745}}, \\
A(18327456) &= -\frac{n_{75}}{s_{183}s_{745}} + \frac{n_{76}}{s_{183}s_{456}} - \frac{n_{80}}{s_{183}s_{274}} - \frac{n_{123}}{s_{274}s_{561}} - \frac{n_{124}}{s_{561}s_{832}} - \frac{n_{125}}{s_{327}s_{561}} \\
&\quad + \frac{n_{145}}{s_{618}s_{745}} - \frac{n_{149}}{s_{274}s_{618}} + \frac{n_{151}}{s_{327}s_{618}} - \frac{n_{176}}{s_{327}s_{456}} + \frac{n_{179}}{s_{745}s_{832}} - \frac{n_{180}}{s_{456}s_{832}}, \\
A(18327654) &= -\frac{n_{73}}{s_{183}s_{765}} - \frac{n_{76}}{s_{183}s_{654}} - \frac{n_{77}}{s_{183}s_{276}} - \frac{n_{87}}{s_{276}s_{541}} - \frac{n_{88}}{s_{541}s_{832}} - \frac{n_{89}}{s_{327}s_{541}} \\
&\quad + \frac{n_{109}}{s_{418}s_{765}} - \frac{n_{112}}{s_{276}s_{418}} + \frac{n_{115}}{s_{327}s_{418}} + \frac{n_{176}}{s_{327}s_{654}} + \frac{n_{177}}{s_{765}s_{832}} + \frac{n_{180}}{s_{654}s_{832}}, \\
A(18347256) &= -\frac{n_{78}}{s_{183}s_{725}} + \frac{n_{79}}{s_{183}s_{256}} + \frac{n_{80}}{s_{183}s_{472}} - \frac{n_{120}}{s_{561}s_{834}} - \frac{n_{121}}{s_{347}s_{561}} + \frac{n_{123}}{s_{472}s_{561}} \\
&\quad + \frac{n_{146}}{s_{347}s_{618}} + \frac{n_{148}}{s_{618}s_{725}} + \frac{n_{149}}{s_{472}s_{618}} - \frac{n_{191}}{s_{256}s_{834}} - \frac{n_{192}}{s_{256}s_{347}} + \frac{n_{194}}{s_{725}s_{834}}, \\
A(18347652) &= -\frac{n_{21}}{s_{476}s_{521}} - \frac{n_{25}}{s_{521}s_{834}} - \frac{n_{26}}{s_{347}s_{521}} + \frac{n_{46}}{s_{218}s_{765}} - \frac{n_{47}}{s_{218}s_{476}} + \frac{n_{52}}{s_{218}s_{347}} \\
&\quad + \frac{n_{73}}{s_{183}s_{765}} - \frac{n_{74}}{s_{183}s_{476}} - \frac{n_{79}}{s_{183}s_{652}} + \frac{n_{191}}{s_{652}s_{834}} + \frac{n_{192}}{s_{347}s_{652}} + \frac{n_{211}}{s_{765}s_{834}}, \\
A(18367254) &= \frac{n_{77}}{s_{183}s_{672}} + \frac{n_{78}}{s_{183}s_{725}} + \frac{n_{81}}{s_{183}s_{254}} - \frac{n_{84}}{s_{541}s_{836}} - \frac{n_{85}}{s_{367}s_{541}} + \frac{n_{87}}{s_{541}s_{672}} \\
&\quad + \frac{n_{110}}{s_{367}s_{418}} + \frac{n_{112}}{s_{418}s_{672}} + \frac{n_{113}}{s_{418}s_{725}} - \frac{n_{183}}{s_{254}s_{836}} - \frac{n_{184}}{s_{254}s_{367}} + \frac{n_{193}}{s_{725}s_{836}}, \\
A(18367452) &= \frac{n_{21}}{s_{521}s_{674}} - \frac{n_{23}}{s_{521}s_{836}} - \frac{n_{24}}{s_{367}s_{521}} + \frac{n_{47}}{s_{218}s_{674}} + \frac{n_{48}}{s_{218}s_{745}} + \frac{n_{50}}{s_{218}s_{367}} \\
&\quad + \frac{n_{74}}{s_{183}s_{674}} + \frac{n_{75}}{s_{183}s_{745}} - \frac{n_{81}}{s_{183}s_{452}} + \frac{n_{183}}{s_{452}s_{836}} + \frac{n_{184}}{s_{367}s_{452}} + \frac{n_{215}}{s_{745}s_{836}}, \\
A(12543876) &= -\frac{n_{19}}{s_{125}s_{876}} - \frac{n_{22}}{s_{125}s_{387}} - \frac{n_{25}}{s_{125}s_{438}} + \frac{n_{32}}{s_{387}s_{612}} - \frac{n_{34}}{s_{438}s_{612}} + \frac{n_{36}}{s_{543}s_{612}} \\
&\quad - \frac{n_{138}}{s_{438}s_{761}} + \frac{n_{139}}{s_{543}s_{761}} + \frac{n_{141}}{s_{254}s_{761}} + \frac{n_{181}}{s_{254}s_{876}} + \frac{n_{182}}{s_{254}s_{387}} - \frac{n_{208}}{s_{543}s_{876}},
\end{aligned}$$

$$\begin{aligned}
A(12563478) &= \frac{n_{20}}{s_{125}s_{478}} - \frac{n_{26}}{s_{125}s_{347}} + \frac{n_{27}}{s_{125}s_{634}} + \frac{n_{51}}{s_{563}s_{812}} + \frac{n_{52}}{s_{347}s_{812}} - \frac{n_{53}}{s_{634}s_{812}} \\
&\quad + \frac{n_{155}}{s_{563}s_{781}} + \frac{n_{156}}{s_{634}s_{781}} + \frac{n_{158}}{s_{256}s_{781}} - \frac{n_{189}}{s_{256}s_{478}} + \frac{n_{192}}{s_{256}s_{347}} + \frac{n_{212}}{s_{478}s_{563}}, \\
A(12563874) &= \frac{n_{14}}{s_{387}s_{412}} - \frac{n_{15}}{s_{412}s_{638}} + \frac{n_{18}}{s_{412}s_{563}} - \frac{n_{20}}{s_{125}s_{874}} + \frac{n_{22}}{s_{125}s_{387}} - \frac{n_{23}}{s_{125}s_{638}} \\
&\quad - \frac{n_{101}}{s_{638}s_{741}} + \frac{n_{103}}{s_{563}s_{741}} + \frac{n_{105}}{s_{256}s_{741}} + \frac{n_{189}}{s_{256}s_{874}} + \frac{n_{190}}{s_{256}s_{387}} - \frac{n_{212}}{s_{563}s_{874}}, \\
A(12583476) &= \frac{n_{21}}{s_{125}s_{476}} + \frac{n_{25}}{s_{125}s_{834}} + \frac{n_{26}}{s_{125}s_{347}} + \frac{n_{33}}{s_{583}s_{612}} + \frac{n_{34}}{s_{612}s_{834}} + \frac{n_{35}}{s_{347}s_{612}} \\
&\quad - \frac{n_{137}}{s_{583}s_{761}} + \frac{n_{138}}{s_{761}s_{834}} + \frac{n_{140}}{s_{258}s_{761}} + \frac{n_{196}}{s_{258}s_{476}} + \frac{n_{198}}{s_{258}s_{347}} + \frac{n_{213}}{s_{476}s_{583}}, \\
A(12583674) &= \frac{n_{15}}{s_{412}s_{836}} + \frac{n_{16}}{s_{367}s_{412}} + \frac{n_{17}}{s_{412}s_{583}} - \frac{n_{21}}{s_{125}s_{674}} + \frac{n_{23}}{s_{125}s_{836}} + \frac{n_{24}}{s_{125}s_{367}} \\
&\quad + \frac{n_{101}}{s_{741}s_{836}} - \frac{n_{102}}{s_{583}s_{741}} + \frac{n_{104}}{s_{258}s_{741}} - \frac{n_{196}}{s_{258}s_{674}} + \frac{n_{197}}{s_{258}s_{367}} - \frac{n_{213}}{s_{583}s_{674}}, \\
A(14523678) &= \frac{n_{82}}{s_{145}s_{678}} - \frac{n_{85}}{s_{145}s_{367}} - \frac{n_{90}}{s_{145}s_{236}} + \frac{n_{110}}{s_{367}s_{814}} + \frac{n_{116}}{s_{236}s_{814}} + \frac{n_{117}}{s_{523}s_{814}} \\
&\quad - \frac{n_{159}}{s_{452}s_{781}} - \frac{n_{160}}{s_{236}s_{781}} + \frac{n_{161}}{s_{523}s_{781}} + \frac{n_{167}}{s_{523}s_{678}} + \frac{n_{181}}{s_{452}s_{678}} - \frac{n_{184}}{s_{367}s_{452}}, \\
A(14523876) &= -\frac{n_{82}}{s_{145}s_{876}} - \frac{n_{83}}{s_{145}s_{387}} - \frac{n_{88}}{s_{145}s_{238}} + \frac{n_{92}}{s_{387}s_{614}} - \frac{n_{97}}{s_{238}s_{614}} + \frac{n_{99}}{s_{523}s_{614}} \\
&\quad - \frac{n_{141}}{s_{452}s_{761}} - \frac{n_{142}}{s_{238}s_{761}} + \frac{n_{143}}{s_{523}s_{761}} - \frac{n_{167}}{s_{523}s_{876}} - \frac{n_{181}}{s_{452}s_{876}} - \frac{n_{182}}{s_{387}s_{452}}, \\
A(14563278) &= \frac{n_{86}}{s_{145}s_{278}} - \frac{n_{89}}{s_{145}s_{327}} + \frac{n_{90}}{s_{145}s_{632}} + \frac{n_{111}}{s_{563}s_{814}} + \frac{n_{115}}{s_{327}s_{814}} - \frac{n_{116}}{s_{632}s_{814}} \\
&\quad + \frac{n_{154}}{s_{456}s_{781}} - \frac{n_{155}}{s_{563}s_{781}} + \frac{n_{160}}{s_{632}s_{781}} + \frac{n_{176}}{s_{327}s_{456}} - \frac{n_{204}}{s_{278}s_{456}} + \frac{n_{205}}{s_{278}s_{563}}, \\
A(14563872) &= -\frac{n_{14}}{s_{214}s_{387}} + \frac{n_{15}}{s_{214}s_{638}} - \frac{n_{18}}{s_{214}s_{563}} + \frac{n_{39}}{s_{456}s_{721}} - \frac{n_{40}}{s_{638}s_{721}} + \frac{n_{42}}{s_{563}s_{721}} \\
&\quad + \frac{n_{83}}{s_{145}s_{387}} - \frac{n_{84}}{s_{145}s_{638}} - \frac{n_{86}}{s_{145}s_{872}} + \frac{n_{204}}{s_{456}s_{872}} - \frac{n_{205}}{s_{563}s_{872}} + \frac{n_{216}}{s_{387}s_{456}}, \\
A(14583276) &= \frac{n_{87}}{s_{145}s_{276}} + \frac{n_{88}}{s_{145}s_{832}} + \frac{n_{89}}{s_{145}s_{327}} + \frac{n_{93}}{s_{583}s_{614}} + \frac{n_{97}}{s_{614}s_{832}} + \frac{n_{98}}{s_{327}s_{614}} \\
&\quad + \frac{n_{136}}{s_{458}s_{761}} + \frac{n_{137}}{s_{583}s_{761}} + \frac{n_{142}}{s_{761}s_{832}} + \frac{n_{175}}{s_{327}s_{458}} + \frac{n_{200}}{s_{276}s_{458}} + \frac{n_{201}}{s_{276}s_{583}}, \\
A(14583672) &= -\frac{n_{15}}{s_{214}s_{836}} - \frac{n_{16}}{s_{214}s_{367}} - \frac{n_{17}}{s_{214}s_{583}} + \frac{n_{38}}{s_{458}s_{721}} + \frac{n_{40}}{s_{721}s_{836}} - \frac{n_{41}}{s_{583}s_{721}} \\
&\quad + \frac{n_{84}}{s_{145}s_{836}} + \frac{n_{85}}{s_{145}s_{367}} - \frac{n_{87}}{s_{145}s_{672}} - \frac{n_{200}}{s_{458}s_{672}} - \frac{n_{201}}{s_{583}s_{672}} + \frac{n_{214}}{s_{367}s_{458}}. \tag{25}
\end{aligned}$$

## B Generalized Jacobi relations

To enforce the duality between color and kinematics, we impose the generalized Jacobi relations between the numerators. Under the color-kinematic duality, 57 of these numerators form an independent basis. We present the set of generalized Jacobi relations necessary to solve for a set of 57 basis numerators. Once the relations are solved, the dependent numerators are substituted into equation (25) to yield equations relating basis amplitudes to basis numerators.

$$\begin{aligned}
n_1 - n_7 + n_8 + n_9 &= 0, & n_3 - n_5 + n_6 - n_8 &= 0, & -n_3 + n_4 + n_5 - n_9 &= 0, \\
-n_1 - n_4 - n_6 + n_7 &= 0, & n_2 + n_3 + n_6 - n_7 &= 0, & n_1 - n_2 - n_5 + n_9 &= 0, \\
n_{19} - n_{25} + n_{26} + n_{27} &= 0, & -n_{20} + n_{21} + n_{23} - n_{26} &= 0, & n_{20} - n_{23} + n_{24} - n_{27} &= 0, \\
-n_{19} - n_{21} - n_{24} + n_{25} &= 0, & n_{21} + n_{22} + n_{23} - n_{25} &= 0, & n_{19} - n_{20} - n_{22} + n_{27} &= 0, \\
n_{37} - n_{43} + n_{44} - n_{45} &= 0, & -n_{38} + n_{39} + n_{40} + n_{45} &= 0, & n_{38} - n_{40} - n_{42} - n_{44} &= 0, \\
-n_{37} - n_{39} + n_{42} + n_{43} &= 0, & n_{39} + n_{40} + n_{41} - n_{43} &= 0, & n_{37} - n_{38} - n_{41} + n_{44} &= 0, \\
n_{99} + n_{108} - n_{117} + n_{167} &= 0, & -n_{108} + n_{152} - n_{168} + n_{169} &= 0, & -n_{99} + n_{143} - n_{152} + n_{168} &= 0, \\
n_{117} - n_{143} - n_{167} - n_{169} &= 0, & -n_{117} + n_{152} + n_{161} + n_{169} &= 0, & n_{99} - n_{161} + n_{167} - n_{168} &= 0, \\
-n_{89} + n_{98} - n_{115} + n_{174} &= 0, & n_{89} + n_{151} - n_{175} + n_{176} &= 0, & -n_{98} - n_{125} - n_{151} + n_{175} &= 0, \\
n_{115} + n_{125} - n_{174} - n_{176} &= 0, & -n_{115} + n_{133} + n_{151} + n_{176} &= 0, & n_{98} - n_{133} + n_{174} - n_{175} &= 0, \\
n_{11} + n_{12} - n_{16} + n_{17} &= 0, & n_{10} - n_{11} + n_{14} - n_{18} &= 0, & -n_{13} + n_{14} + n_{15} - n_{17} &= 0, \\
-n_{12} + n_{13} - n_{14} + n_{18} &= 0, & -n_{10} - n_{13} + n_{16} - n_{17} &= 0, & -n_{11} - n_{15} + n_{16} - n_{18} &= 0, \\
n_{135} - n_{144} + n_{164} + n_{165} &= 0, & -n_{126} + n_{162} + n_{163} - n_{164} &= 0, & -n_{135} + n_{153} + n_{162} - n_{166} &= 0, \\
n_{126} - n_{162} - n_{165} + n_{166} &= 0, & -n_{135} + n_{144} - n_{163} - n_{166} &= 0, & -n_{126} + n_{144} - n_{153} - n_{164} &= 0, \\
n_{81} - n_{141} + n_{182} + n_{183} &= 0, & -n_{72} + n_{159} + n_{181} - n_{182} &= 0, & -n_{81} + n_{150} + n_{159} - n_{184} &= 0, \\
n_{72} - n_{159} - n_{183} + n_{184} &= 0, & -n_{81} + n_{141} - n_{181} - n_{184} &= 0, & -n_{72} + n_{141} - n_{150} - n_{182} &= 0, \\
n_{80} - n_{123} + n_{186} + n_{187} &= 0, & -n_{71} + n_{132} + n_{185} - n_{187} &= 0, & -n_{80} + n_{132} + n_{149} - n_{188} &= 0,
\end{aligned}$$

$$\begin{aligned}
& n_{71} - n_{132} - n_{186} + n_{188} = 0, & -n_{80} + n_{123} - n_{185} - n_{188} = 0, & -n_{71} + n_{123} - n_{149} - n_{187} = 0, \\
& -n_{62} + n_{96} - n_{113} + n_{193} = 0, & n_{62} + n_{148} - n_{194} + n_{195} = 0, & -n_{70} - n_{96} - n_{148} + n_{194} = 0, \\
& n_{70} + n_{113} - n_{193} - n_{195} = 0, & n_{78} - n_{113} + n_{148} + n_{195} = 0, & -n_{78} + n_{96} + n_{193} - n_{194} = 0, \\
& n_{28} + n_{30} + n_{33} - n_{35} = 0, & -n_{28} + n_{29} + n_{32} - n_{36} = 0, & -n_{31} + n_{32} - n_{33} + n_{34} = 0, \\
& -n_{30} + n_{31} - n_{32} + n_{36} = 0, & -n_{29} - n_{31} - n_{33} + n_{35} = 0, & -n_{28} - n_{34} + n_{35} - n_{36} = 0, \\
& -n_{107} + n_{134} + n_{170} + n_{172} = 0, & -n_{90} + n_{160} - n_{170} + n_{171} = 0, & n_{116} - n_{134} + n_{160} - n_{173} = 0, \\
& n_{90} - n_{160} - n_{172} + n_{173} = 0, & n_{107} - n_{134} - n_{171} - n_{173} = 0, & -n_{90} + n_{107} - n_{116} - n_{170} = 0, \\
& n_{79} - n_{105} + n_{190} + n_{191} = 0, & -n_{63} + n_{158} + n_{189} - n_{190} = 0, & -n_{79} + n_{114} + n_{158} - n_{192} = 0, \\
& n_{63} - n_{158} - n_{191} + n_{192} = 0, & -n_{79} + n_{105} - n_{189} - n_{192} = 0, & -n_{63} + n_{105} - n_{114} - n_{190} = 0, \\
& n_{77} - n_{87} + n_{201} + n_{202} = 0, & -n_{60} + n_{131} + n_{200} - n_{201} = 0, & -n_{77} + n_{112} + n_{131} - n_{203} = 0, \\
& n_{60} - n_{131} - n_{202} + n_{203} = 0, & -n_{77} + n_{87} - n_{200} - n_{203} = 0, & -n_{60} + n_{87} - n_{112} - n_{201} = 0, \\
& n_{46} - n_{49} + n_{51} - n_{52} = 0, & -n_{46} - n_{47} + n_{50} - n_{54} = 0, & -n_{48} + n_{50} - n_{51} - n_{53} = 0, \\
& n_{48} + n_{49} - n_{50} + n_{54} = 0, & n_{47} - n_{48} - n_{51} + n_{52} = 0, & -n_{46} + n_{52} + n_{53} - n_{54} = 0, \\
& -n_{106} + n_{124} + n_{177} - n_{180} = 0, & -n_{88} + n_{142} - n_{177} - n_{178} = 0, & -n_{97} - n_{124} + n_{142} - n_{179} = 0, \\
& n_{88} - n_{142} + n_{179} + n_{180} = 0, & n_{106} - n_{124} + n_{178} - n_{179} = 0, & -n_{88} + n_{97} + n_{106} - n_{177} = 0, \\
& n_{69} - n_{104} + n_{197} - n_{199} = 0, & -n_{61} + n_{140} - n_{196} - n_{197} = 0, & -n_{69} - n_{95} + n_{140} - n_{198} = 0, \\
& n_{61} - n_{140} + n_{198} + n_{199} = 0, & -n_{69} + n_{104} + n_{196} - n_{198} = 0, & -n_{61} + n_{95} + n_{104} - n_{197} = 0, \\
& n_{68} - n_{86} + n_{205} - n_{206} = 0, & -n_{59} + n_{122} - n_{204} - n_{205} = 0, & -n_{68} - n_{94} + n_{122} - n_{207} = 0, \\
& n_{59} - n_{122} + n_{206} + n_{207} = 0, & -n_{68} + n_{86} + n_{204} - n_{207} = 0, & -n_{59} + n_{86} + n_{94} - n_{205} = 0, \\
& n_{55} - n_{61} + n_{62} + n_{63} = 0, & n_{57} - n_{59} + n_{60} - n_{62} = 0, & -n_{57} + n_{58} + n_{59} - n_{63} = 0, \\
& -n_{55} - n_{58} - n_{60} + n_{61} = 0, & n_{56} + n_{57} + n_{60} - n_{61} = 0, & n_{55} - n_{56} - n_{59} + n_{63} = 0, \\
& n_{82} - n_{88} + n_{89} + n_{90} = 0, & n_{84} - n_{86} + n_{87} - n_{89} = 0, & -n_{84} + n_{85} + n_{86} - n_{90} = 0, \\
& -n_{82} - n_{85} - n_{87} + n_{88} = 0, & n_{83} + n_{84} + n_{87} - n_{88} = 0, & n_{82} - n_{83} - n_{86} + n_{90} = 0, \\
& n_{100} - n_{106} + n_{107} - n_{108} = 0, & n_{101} - n_{104} + n_{105} + n_{108} = 0, & -n_{101} - n_{103} + n_{104} - n_{107} = 0,
\end{aligned}$$



$$\begin{aligned}
& -n_{100} + n_{103} - n_{105} + n_{106} = 0, & n_{101} + n_{102} + n_{105} - n_{106} = 0, & n_{100} - n_{102} - n_{104} + n_{107} = 0, \\
& n_{36} + n_{45} - n_{54} + n_{208} = 0, & -n_{45} + n_{147} + n_{203} - n_{207} = 0, & -n_{36} + n_{139} - n_{147} + n_{207} = 0, \\
& n_{54} - n_{139} - n_{203} - n_{208} = 0, & -n_{54} + n_{147} + n_{157} + n_{203} = 0, & n_{36} - n_{157} - n_{207} + n_{208} = 0, \\
& -n_{26} + n_{35} - n_{52} + n_{210} = 0, & n_{26} + n_{146} + n_{192} - n_{198} = 0, & -n_{35} - n_{121} - n_{146} + n_{198} = 0, \\
& n_{52} + n_{121} - n_{192} - n_{210} = 0, & -n_{52} + n_{129} + n_{146} + n_{192} = 0, & n_{35} - n_{129} - n_{198} + n_{210} = 0, \\
& -n_8 + n_{31} - n_{48} + n_{215} = 0, & n_8 + n_{145} + n_{173} - n_{179} = 0, & -n_{31} - n_{67} - n_{145} + n_{179} = 0, \\
& n_{48} + n_{67} - n_{173} - n_{215} = 0, & -n_{48} + n_{75} + n_{145} + n_{173} = 0, & n_{31} - n_{75} - n_{179} + n_{215} = 0, \\
& n_{91} + n_{93} + n_{95} - n_{98} = 0, & -n_{91} + n_{92} + n_{94} - n_{99} = 0, & n_{92} - n_{93} - n_{96} + n_{97} = 0, \\
& -n_{92} - n_{95} + n_{96} + n_{99} = 0, & -n_{93} - n_{94} - n_{96} + n_{98} = 0, & -n_{91} - n_{97} + n_{98} - n_{99} = 0, \\
& -n_{44} + n_{130} + n_{199} + n_{209} = 0, & -n_{27} + n_{156} + n_{206} - n_{209} = 0, & n_{53} - n_{130} + n_{156} - n_{195} = 0, \\
& n_{27} - n_{156} + n_{195} - n_{199} = 0, & n_{44} - n_{130} - n_{195} - n_{206} = 0, & -n_{27} + n_{44} - n_{53} - n_{209} = 0, \\
& -n_{39} + n_{76} + n_{180} + n_{216} = 0, & -n_9 + n_{154} + n_{204} - n_{216} = 0, & n_{49} - n_{76} + n_{154} - n_{176} = 0, \\
& n_9 - n_{154} + n_{176} - n_{180} = 0, & n_{39} - n_{76} - n_{176} - n_{204} = 0, & -n_9 + n_{39} - n_{49} - n_{216} = 0, \\
& -n_{21} + n_{74} + n_{178} + n_{213} = 0, & -n_6 + n_{127} + n_{196} - n_{213} = 0, & n_{47} - n_{74} + n_{127} - n_{169} = 0, \\
& n_6 - n_{127} + n_{169} - n_{178} = 0, & n_{21} - n_{74} - n_{169} - n_{196} = 0, & -n_6 + n_{21} - n_{47} - n_{213} = 0, \\
& n_{109} + n_{111} - n_{114} - n_{115} = 0, & -n_{109} + n_{110} - n_{112} - n_{117} = 0, & n_{110} - n_{111} - n_{113} - n_{116} = 0, \\
& -n_{110} + n_{113} + n_{114} + n_{117} = 0, & -n_{111} + n_{112} - n_{113} + n_{115} = 0, & -n_{109} + n_{115} + n_{116} - n_{117} = 0, \\
& -n_{43} + n_{120} - n_{191} + n_{211} = 0, & -n_{25} + n_{138} - n_{202} - n_{211} = 0, & -n_{34} - n_{120} + n_{138} - n_{194} = 0, \\
& n_{25} - n_{138} + n_{191} + n_{194} = 0, & n_{43} - n_{120} - n_{194} + n_{202} = 0, & -n_{25} + n_{34} + n_{43} - n_{211} = 0, \\
& -n_{38} + n_{66} - n_{172} + n_{214} = 0, & -n_7 + n_{136} - n_{200} - n_{214} = 0, & -n_{30} - n_{66} + n_{136} - n_{175} = 0, \\
& n_7 - n_{136} + n_{172} + n_{175} = 0, & n_{38} - n_{66} - n_{175} + n_{200} = 0, & -n_7 + n_{30} + n_{38} - n_{214} = 0, \\
& -n_{20} + n_{65} - n_{171} + n_{212} = 0, & -n_5 + n_{118} - n_{189} - n_{212} = 0, & -n_{29} - n_{65} + n_{118} - n_{168} = 0, \\
& n_5 - n_{118} + n_{168} + n_{171} = 0, & n_{20} - n_{65} - n_{168} + n_{189} = 0, & -n_5 + n_{20} + n_{29} - n_{212} = 0, \\
& n_{65} - n_{69} + n_{70} + n_{72} = 0, & n_{66} - n_{68} - n_{70} + n_{71} = 0, & -n_{66} + n_{67} + n_{68} - n_{72} = 0,
\end{aligned}$$

$$\begin{aligned}
& -n_{65} - n_{67} + n_{69} - n_{71} = 0, & n_{64} + n_{66} - n_{69} + n_{71} = 0, & -n_{64} + n_{65} - n_{68} + n_{72} = 0, \\
& n_{118} - n_{124} + n_{125} + n_{126} = 0, & n_{120} - n_{122} + n_{123} - n_{125} = 0, & -n_{120} + n_{121} + n_{122} - n_{126} = 0, \\
& -n_{118} - n_{121} - n_{123} + n_{124} = 0, & n_{119} + n_{120} + n_{123} - n_{124} = 0, & n_{118} - n_{119} - n_{122} + n_{126} = 0, \\
& n_{136} - n_{142} - n_{143} + n_{144} = 0, & n_{138} - n_{140} + n_{141} + n_{143} = 0, & -n_{138} - n_{139} + n_{140} - n_{144} = 0, \\
& -n_{136} + n_{139} - n_{141} + n_{142} = 0, & n_{137} + n_{138} + n_{141} - n_{142} = 0, & n_{136} - n_{137} - n_{140} + n_{144} = 0, \\
& n_{18} + n_{42} - n_{51} + n_{212} = 0, & -n_{42} + n_{111} + n_{188} - n_{205} = 0, & -n_{18} + n_{103} - n_{111} + n_{205} = 0, \\
& n_{51} - n_{103} - n_{188} - n_{212} = 0, & -n_{51} + n_{111} + n_{155} + n_{188} = 0, & n_{18} - n_{155} - n_{205} + n_{212} = 0, \\
& n_{16} - n_{24} - n_{50} + n_{214} = 0, & n_{24} + n_{110} + n_{184} - n_{197} = 0, & -n_{16} - n_{85} - n_{110} + n_{197} = 0, \\
& n_{50} + n_{85} - n_{184} - n_{214} = 0, & -n_{50} + n_{110} + n_{128} + n_{184} = 0, & n_{16} - n_{128} - n_{197} + n_{214} = 0, \\
& -n_4 + n_{13} - n_{46} + n_{211} = 0, & n_4 + n_{109} + n_{166} - n_{177} = 0, & -n_{13} - n_{58} - n_{109} + n_{177} = 0, \\
& n_{46} + n_{58} - n_{166} - n_{211} = 0, & -n_{46} + n_{73} + n_{109} + n_{166} = 0, & n_{13} - n_{73} - n_{177} + n_{211} = 0, \\
& n_{145} + n_{147} - n_{150} - n_{151} = 0, & -n_{145} + n_{146} - n_{149} - n_{152} = 0, & n_{146} - n_{147} - n_{148} - n_{153} = 0, \\
& -n_{146} + n_{148} + n_{150} + n_{152} = 0, & -n_{147} - n_{148} + n_{149} + n_{151} = 0, & -n_{145} + n_{151} - n_{152} + n_{153} = 0, \\
& -n_{40} + n_{84} - n_{183} + n_{215} = 0, & -n_{23} + n_{101} - n_{186} - n_{215} = 0, & -n_{15} - n_{84} + n_{101} - n_{193} = 0, \\
& n_{23} - n_{101} + n_{183} + n_{193} = 0, & n_{40} - n_{84} + n_{186} - n_{193} = 0, & n_{15} - n_{23} + n_{40} - n_{215} = 0, \\
& -n_{37} + n_{57} - n_{165} + n_{210} = 0, & -n_3 + n_{100} - n_{185} - n_{210} = 0, & -n_{12} - n_{57} + n_{100} - n_{174} = 0, \\
& n_3 - n_{100} + n_{165} + n_{174} = 0, & n_{37} - n_{57} - n_{174} + n_{185} = 0, & -n_3 + n_{12} + n_{37} - n_{210} = 0, \\
& -n_{19} + n_{55} - n_{163} + n_{208} = 0, & -n_1 + n_{82} - n_{181} - n_{208} = 0, & -n_{10} - n_{55} + n_{82} - n_{167} = 0, \\
& n_1 - n_{82} + n_{163} + n_{167} = 0, & n_{19} - n_{55} - n_{167} + n_{181} = 0, & -n_1 + n_{10} + n_{19} - n_{208} = 0, \\
& n_{74} - n_{78} - n_{79} + n_{81} = 0, & n_{76} - n_{77} + n_{78} + n_{80} = 0, & -n_{75} - n_{76} + n_{77} - n_{81} = 0, \\
& -n_{74} + n_{75} + n_{79} - n_{80} = 0, & -n_{73} + n_{76} - n_{79} + n_{80} = 0, & n_{73} + n_{74} - n_{77} + n_{81} = 0, \\
& n_{127} - n_{133} - n_{134} + n_{135} = 0, & n_{130} - n_{131} + n_{132} + n_{133} = 0, & -n_{129} - n_{130} + n_{131} - n_{135} = 0, \\
& -n_{127} + n_{129} - n_{132} + n_{134} = 0, & -n_{128} + n_{130} + n_{132} - n_{134} = 0, & n_{127} + n_{128} - n_{131} + n_{135} = 0, \\
& n_{154} - n_{160} - n_{161} + n_{162} = 0, & n_{156} - n_{158} + n_{159} + n_{161} = 0, & -n_{156} - n_{157} + n_{158} - n_{162} = 0,
\end{aligned}$$

$$\begin{aligned}
& -n_{154} + n_{157} - n_{159} + n_{160} = 0, & -n_{155} + n_{156} + n_{159} - n_{160} = 0, & n_{154} + n_{155} - n_{158} + n_{162} = 0, \\
& n_{17} - n_{33} - n_{41} + n_{213} = 0, & n_{41} + n_{93} + n_{187} - n_{201} = 0, & -n_{17} - n_{93} - n_{102} + n_{201} = 0, \\
& n_{33} + n_{102} - n_{187} - n_{213} = 0, & -n_{33} + n_{93} - n_{137} + n_{187} = 0, & n_{17} + n_{137} - n_{201} + n_{213} = 0, \\
& n_{14} - n_{22} - n_{32} + n_{216} = 0, & n_{22} + n_{92} + n_{182} - n_{190} = 0, & -n_{14} - n_{83} - n_{92} + n_{190} = 0, \\
& n_{32} + n_{83} - n_{182} - n_{216} = 0, & -n_{32} + n_{92} - n_{119} + n_{182} = 0, & n_{14} + n_{119} - n_{190} + n_{216} = 0, \\
& -n_2 + n_{11} - n_{28} + n_{209} = 0, & n_2 + n_{91} + n_{164} - n_{170} = 0, & -n_{11} - n_{56} - n_{91} + n_{170} = 0, \\
& n_{28} + n_{56} - n_{164} - n_{209} = 0, & -n_{28} - n_{64} + n_{91} + n_{164} = 0, & n_{11} + n_{64} - n_{170} + n_{209} = 0.
\end{aligned}
\tag{26}$$
